# Supplementary material for: HeteSpaceyWalk: A Heterogeneous Spacey Random Walk for Heterogeneous Information Network Embedding
Source: arXiv:1909.03228 source file (2019-09-07)
Supplement: Supplementary file 1 [file appendix.tex]

%\clearpage
\appendix

\section{More Results}
\label{appendix:more_results}
Due to the lack of space of the paper, we report more experimental results in this supplementary material.

We report the variances of the Micro-F1 scores and the Macro-F1 scores for multi-label node classification in Table~\ref{Tab:MicroF1_var_in_appendix} and Table~\ref{Tab:MacroF1_var_in_appendix},
and report the detailed AUC scores of link prediction for all binary operators on four heterogeneous networks in Table~\ref{Tab:lp_results_ACM_in_appendix}, Table~\ref{Tab:lp_results_DBLP_in_appendix}, Table~\ref{Tab:lp_results_Douban_in_appendix}, and Table~\ref{Tab:lp_results_Yelp_in_appendix}.
Moreover, given meta-path $\mathcal P_2$ and meta-graph $\mathcal S_2$, %(as shown in Figure~\ref{Fig:ACM_dataset}),
we report the parameter sensitivity of different methods for author node classification on the ACM dataset in Figure~\ref{Fig:Parameter_sensitivity_in_appendix}.

\begin{table*}[b]
	\small
	%		\footnotesize
	\caption{\small The variances of the Micro-F1 scores for multi-label node classification. ``--'' indicates that the used meta-path/meta-graph cannot generate embeddings for nodes of target type.}\label{Tab:MicroF1_var_in_appendix}
	\vspace{-0.1in}
	\centering
	\begin{tabular}{p{2.8cm}<{\centering}|p{0.9cm}<{\centering}|p{0.9cm}<{\centering}|p{0.9cm}<{\centering}|p{0.9cm}<{\centering}|p{0.9cm}<{\centering}|p{0.9cm}<{\centering}|p{0.9cm}<{\centering}|p{0.9cm}<{\centering}|p{0.9cm}<{\centering}|p{0.9cm}<{\centering}|p{0.9cm}<{\centering}}
		\toprule
		Dataset & \multicolumn{3}{c|}{ACM} & \multicolumn{2}{c|}{DBLP} & \multicolumn{4}{c|}{Douban} & \multicolumn{2}{c}{Yelp} \\
\midrule
Node Type & Paper & Author & Venue & Paper & Author & User & Movie & Director & Actor & User & Business \\
\midrule
DeepWalk & 
6.56e-6 & 7.67e-6 & 1.07e-5 & 4.79e-4 & 8.69e-6 & 3.19e-6 & 3.01e-6 & 8.83e-6 & 5.00e-6 & 3.10e-6 & 6.13e-7 \\ 
LINE & 
4.82e-5 & 5.27e-6 & 3.23e-5 & 1.27e-4 & 3.49e-7 & 5.73e-6 & 3.03e-6 & 4.62e-6 & 4.83e-6 & 2.86e-6 & 9.64e-6 \\ 
PTE &
1.97e-5 & 1.14e-5 & 6.85e-4 & 6.53e-4 & 3.28e-7 & 2.74e-6 & 8.05e-6 & 8.85e-5 & 2.08e-5 & 8.65e-6 & 9.20e-6 \\ 
\midrule
Metapath2vec-$\mathcal P_{1}$ & 
3.74e-6 & 2.47e-6 & 8.59e-5 & 2.51e-4 & 1.44e-6 & 1.15e-6 & 5.80e-7 & -- & 5.83e-6 & 5.12e-6 & 2.30e-6 \\ 
Metapath2vec-$\mathcal P_{2}$ & 
8.46e-7 & 1.64e-6 & -- & 3.76e-4 & 4.64e-7 & 2.16e-6 & 2.01e-6 & 1.08e-5 & -- & 1.46e-5 & 2.19e-6 \\ 
\hline	
Metagraph2vec-$\mathcal S_{1}$ &
5.21e-7 & 1.30e-6 & 8.30e-5 & 2.19e-4 & 2.24e-6 & 3.33e-6 & 9.71e-7 & 9.57e-6 & 1.10e-6 & 4.01e-6 & 1.54e-6 \\ 
Metagraph2vec-$\mathcal S_{2}$ &
2.15e-6 & 1.45e-6 & 9.66e-5 & 2.15e-4 & 2.53e-7 & 2.58e-6 & 1.66e-6 & 8.74e-6 & 6.26e-6 & 1.26e-6 & 1.29e-6 \\ 
\midrule
SpaceyMetapath-$\mathcal P_{1}$ &
4.56e-6 & 3.63e-6 & 1.12e-5 & 1.24e-4 & 2.74e-6 & 4.02e-6 & 5.13e-7 & -- & 5.81e-6 & 1.67e-6 & 1.92e-6 \\ 
SpaceyMetapath-$\mathcal P_{2}$ & 
3.84e-6 & 3.56e-6 & -- & 6.18e-4 & 4.20e-6 & 4.25e-6 & 3.06e-6 & 1.05e-5 & -- & 3.99e-6 & 2.15e-6 \\
\hline
SpaceyMetagraph-$\mathcal S_{1}$ & 
6.55e-7 & 2.01e-6 & 3.65e-5 & 1.18e-4 & 2.62e-6 & 1.61e-6 & 9.28e-7 & 4.60e-6 & 1.55e-6 & 8.97e-7 & 3.48e-7 \\ 
SpaceyMetagraph-$\mathcal S_{2}$ & 
2.45e-6 & 2.21e-6 & 3.51e-5 & 3.51e-4 & 8.68e-7 & 1.62e-6 & 7.90e-7 & 6.98e-6 & 5.12e-6 & 9.95e-7 & 7.26e-7 \\
\hline
SpaceyMetaschema &
2.05e-6 & 2.81e-6 & 5.20e-5 & 1.78e-4 & 9.46e-7 & 2.40e-6 & 3.28e-7 & 2.09e-5 & 4.87e-7 & 6.56e-7 & 3.34e-7 \\ 
\bottomrule
	\end{tabular}
%	\vspace{-0.15in}
\end{table*}

\begin{table*}[b]
	\small
	%		\footnotesize
	\caption{\small The variances of the Macro-F1 scores for multi-label node classification. ``--'' indicates that the used meta-path/meta-graph cannot generate embeddings for nodes of target type.}\label{Tab:MacroF1_var_in_appendix}
	\vspace{-0.1in}
	\centering
	\begin{tabular}{p{2.8cm}<{\centering}|p{0.9cm}<{\centering}|p{0.9cm}<{\centering}|p{0.9cm}<{\centering}|p{0.9cm}<{\centering}|p{0.9cm}<{\centering}|p{0.9cm}<{\centering}|p{0.9cm}<{\centering}|p{0.9cm}<{\centering}|p{0.9cm}<{\centering}|p{0.9cm}<{\centering}|p{0.9cm}<{\centering}}
\toprule
Dataset & \multicolumn{3}{c|}{ACM} & \multicolumn{2}{c|}{DBLP} & \multicolumn{4}{c|}{Douban} & \multicolumn{2}{c}{Yelp} \\
\midrule
Node Type & Paper & Author & Venue & Paper & Author & User & Movie & Director & Actor & User & Business \\
\midrule
DeepWalk & 
9.17e-6 & 1.76e-5 & 2.85e-4 & 1.28e-3 & 9.82e-6 & 8.34e-6 & 1.18e-5 & 1.72e-5 & 2.57e-5 & 2.09e-6 & 1.77e-6 \\ 
LINE & 
5.46e-6 & 9.54e-5 & 2.00e-4 & 2.28e-3 & 3.53e-7 & 2.01e-5 & 1.81e-5 & 3.10e-5 & 3.78e-5 & 1.94e-7 & 3.30e-6 \\
PTE &
1.04e-5 & 5.05e-5 & 3.15e-4 & 1.05e-3 & 2.28e-7 & 2.27e-6 & 3.07e-5 & 2.07e-5 & 2.62e-5 & 5.33e-7 & 5.45e-6 \\ 
\midrule
Metapath2vec-$\mathcal P_{1}$ & 
2.65e-6 & 3.76e-6 & 3.04e-4 & 2.66e-4 & 1.70e-6 & 3.04e-5 & 2.78e-6 & -- & 2.21e-5 & 4.19e-6 & 2.05e-6 \\ 
Metapath2vec-$\mathcal P_{2}$ & 
9.80e-6 & 1.02e-5 & -- & 6.07e-4 & 8.29e-7 & 9.00e-5 & 5.41e-6 & 5.53e-5 & -- & 2.90e-6 & 3.10e-6 \\ 
\hline	
Metagraph2vec-$\mathcal S_{1}$ &
1.53e-6 & 2.76e-5 & 1.76e-4 & 2.59e-4 & 2.82e-6 & 6.72e-5 & 7.34e-6 & 4.86e-5 & 1.04e-5 & 6.31e-6 & 8.55e-7 \\ 
Metagraph2vec-$\mathcal S_{2}$ &
6.16e-6 & 1.77e-5 & 6.70e-5 & 4.71e-4 & 2.28e-7 & 4.65e-5 & 1.71e-6 & 7.16e-5 & 2.22e-5 & 1.85e-6 & 1.63e-6 \\ 
\midrule
SpaceyMetapath-$\mathcal P_{1}$ &
2.24e-6 & 4.54e-6 & 2.56e-4 & 2.25e-4 & 3.32e-6 & 7.08e-5 & 5.18e-6 & -- & 3.42e-5 & 2.50e-6 & 8.75e-7 \\ 
SpaceyMetapath-$\mathcal P_{2}$ & 
4.89e-6 & 1.34e-5 & -- & 7.65e-4 & 4.23e-6 & 2.84e-5 & 7.77e-6 & 2.89e-5 & -- & 3.28e-6 & 8.40e-7 \\
\hline
SpaceyMetagraph-$\mathcal S_{1}$ & 
7.39e-6 & 2.63e-5 & 4.21e-4 & 1.86e-4 & 2.82e-6 & 4.62e-5 & 4.93e-6 & 2.72e-5 & 2.84e-5 & 1.98e-6 & 1.02e-6 \\
SpaceyMetagraph-$\mathcal S_{2}$ & 
1.85e-6 & 1.71e-5 & 7.73e-5 & 5.63e-4 & 8.05e-7 & 2.56e-5 & 3.45e-6 & 3.01e-5 & 2.87e-5 & 4.20e-6 & 1.79e-6 \\ 
\hline
SpaceyMetaschema &
8.33e-6 & 1.94e-5 & 1.28e-4 & 3.44e-4 & 1.31e-6 & 5.88e-5 & 9.00e-6 & 5.67e-5 & 1.86e-5 & 1.59e-6 & 6.62e-7 \\ 
\bottomrule
	\end{tabular}
%	\vspace{-0.15in}
\end{table*}

\begin{figure*}[!hbt]
%	\vspace{-0.1in}
	\small
	\setlength{\abovecaptionskip}{-0.05cm}
	\centering
	\subfigure[\small walk-times $w$.]{
		\label{Fig:walk_times_P2}
		\includegraphics[width=0.32\textwidth]{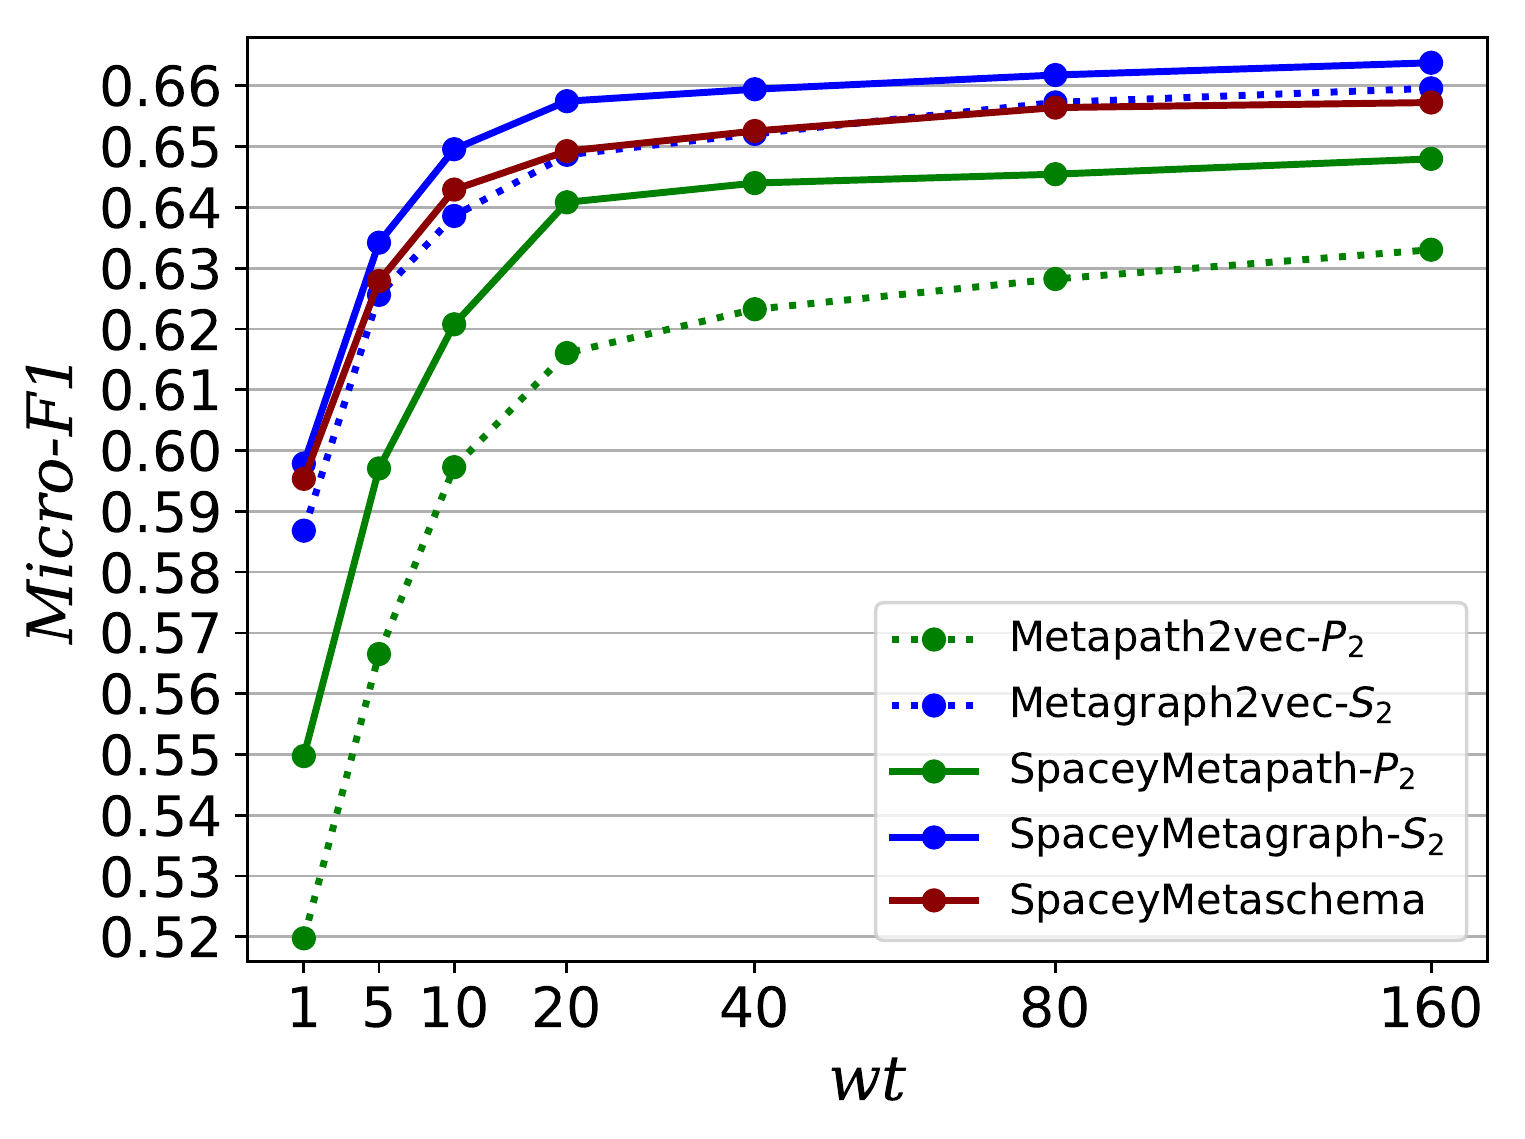}
	}
	%     \hfill
	%	\hspace{0.1in}
	%    \vspace{0.0in}
	\subfigure[\small walk-length $l$.]{
		\label{Fig:walk_length_P2}
		\includegraphics[width=0.32\textwidth]{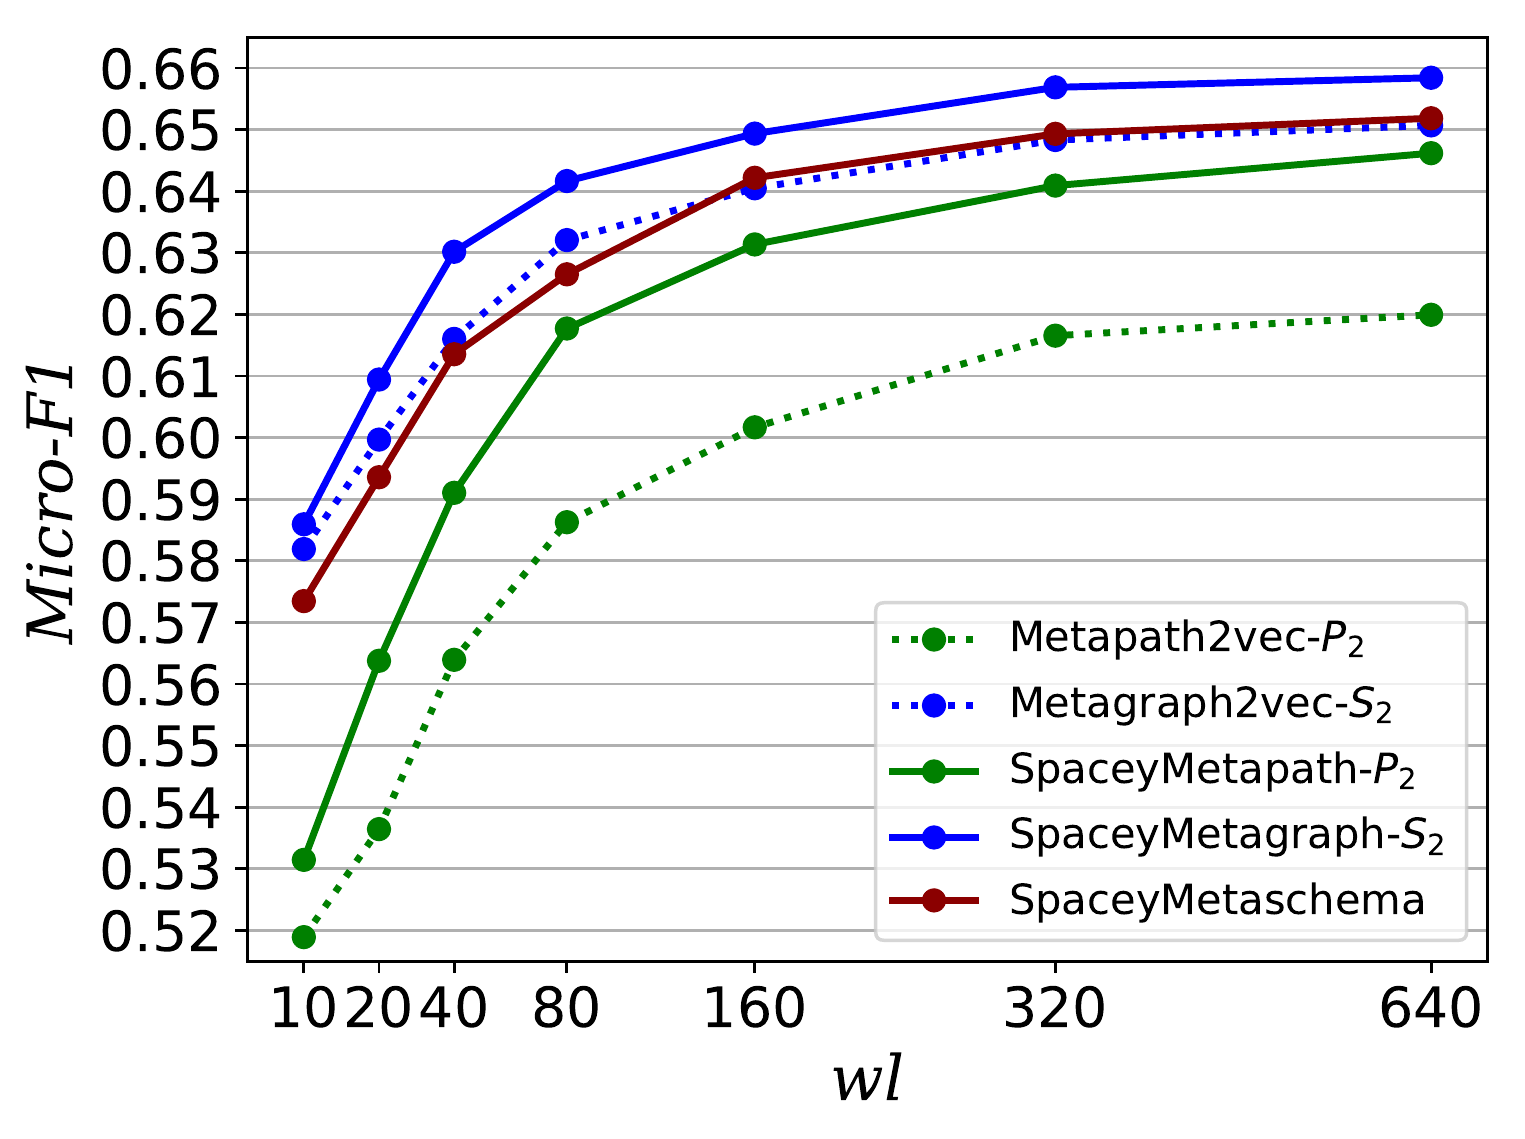}
	}
	%	\hspace{-0.1in}
	%    \vspace{0.in}
	\subfigure[\small personalized-probability $\alpha$.]
	{\label{Fig:personalized_probability_P2}
		\includegraphics[width=0.32\textwidth]{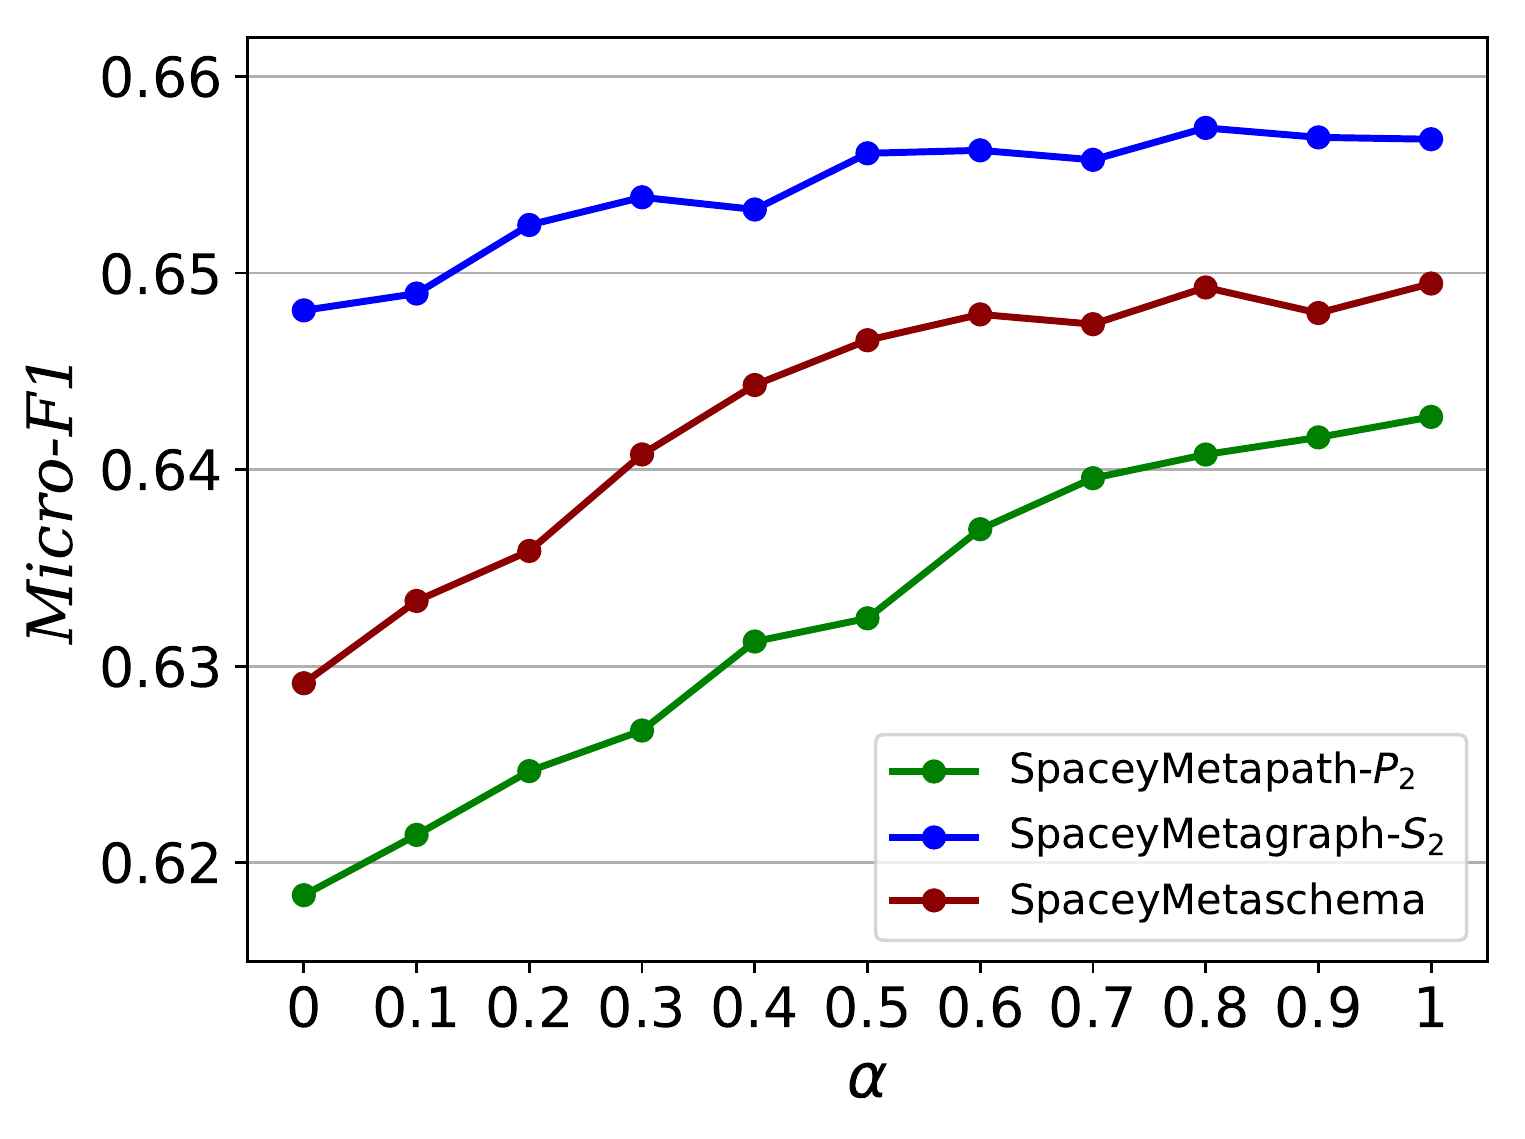}
	}
	%     \hfill
	%	\hspace{0.1in}
	%    \vspace{0.in}
	%	\subfigure[\small scalability analysis.]
	%	{\label{Fig:scalability_time}
	%		\includegraphics[width=0.235\textwidth]{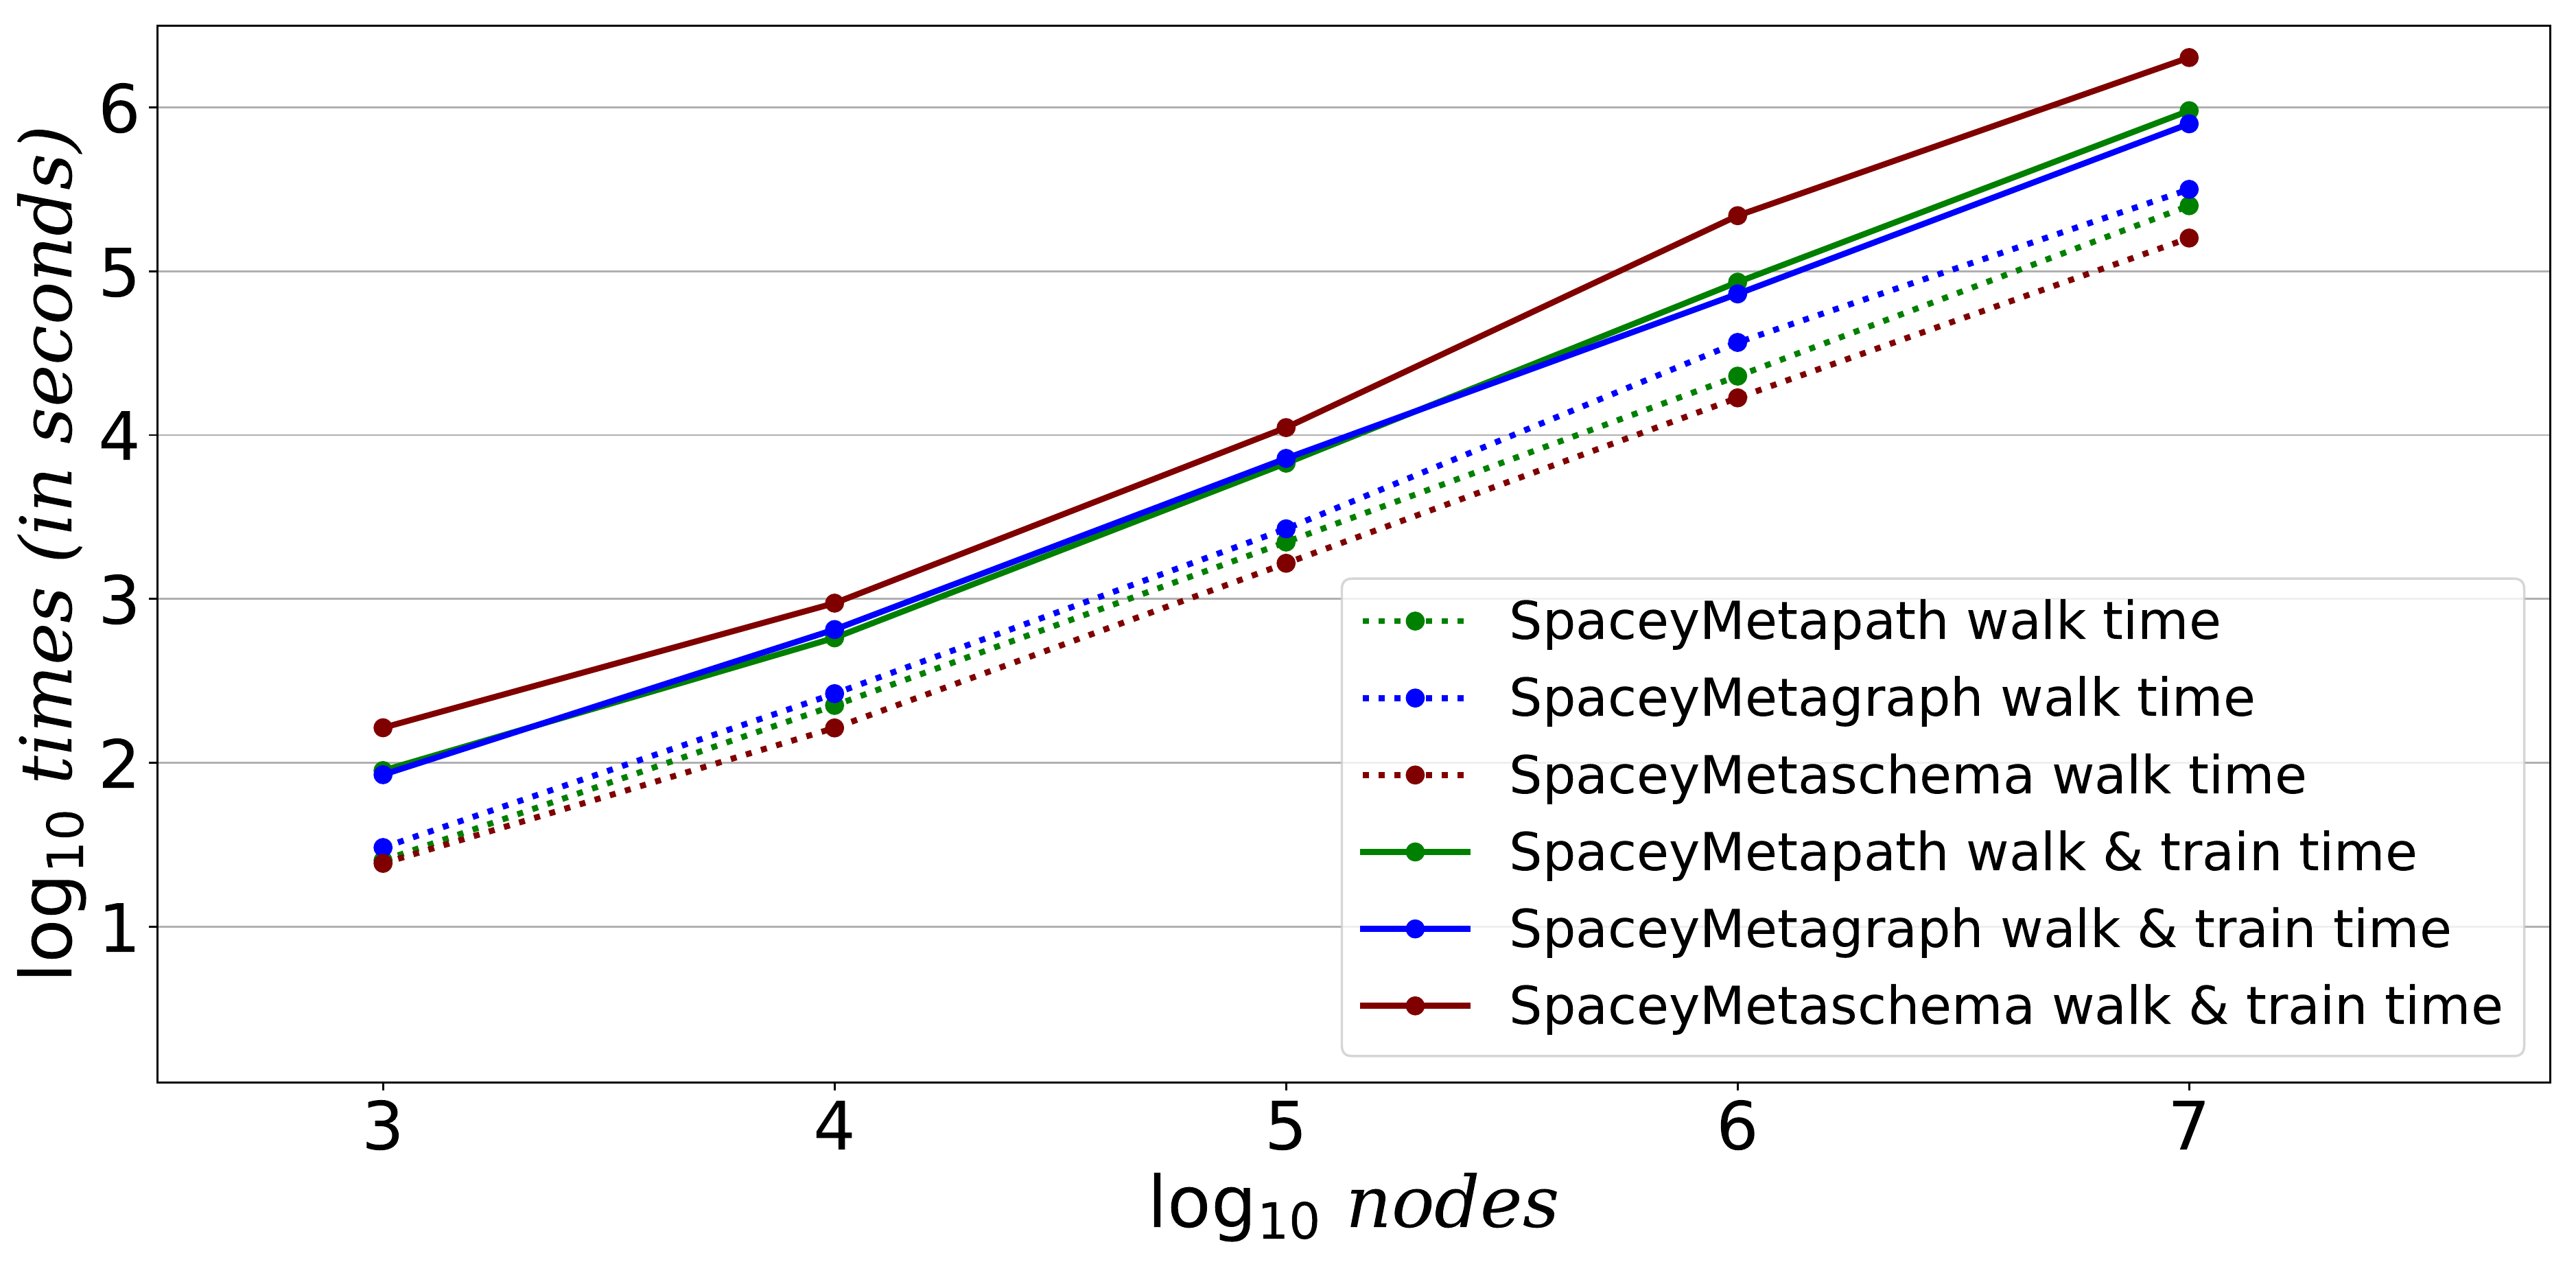}
	%	}
	% \includegraphics[width=0.4\textwidth]{walk-times-author}
	\caption{\small Parameter sensitivity for author node classification on the ACM dataset.}
	\label{Fig:Parameter_sensitivity_in_appendix}
	
\end{figure*}

\begin{table*}[t]
	 	\small
%		\footnotesize
	\caption{\small The AUC scores for link prediction on the ACM dataset. The binary operators: (a) Average, (b) Hadamard, (c)
		Weighted-L1, and (d) Weighted-L2. %are defined in Table~\ref{Tab:binary_operators}. 
		``--'' indicates that the used meta-path/meta-graph cannot generate embeddings for nodes of target type.}\label{Tab:lp_results_ACM_in_appendix}
	\vspace{-0.1in}
	\centering
	\begin{tabular}{p{2.8cm}<{\centering}|p{0.8cm}<{\centering}|p{0.8cm}<{\centering}|p{0.8cm}<{\centering}|p{0.8cm}<{\centering}|p{0.8cm}<{\centering}|p{0.8cm}<{\centering}|p{0.8cm}<{\centering}|p{0.8cm}<{\centering}|p{0.8cm}<{\centering}|p{0.8cm}<{\centering}|p{0.8cm}<{\centering}|p{0.8cm}<{\centering}}
		\toprule
		Edge Type & \multicolumn{4}{c|}{Paper--Paper} & \multicolumn{4}{c|}{Paper--Venue} & \multicolumn{4}{c}{Paper--Term} \\
		\midrule
		Operator & (a) & (b) & (c) & (d) & (a) & (b) & (c) & (d) & (a) & (b) & (c) & (d) \\
		\midrule
		DeepWalk &
		0.6514 & 0.9675 & 0.9270 & 0.9387 & 0.7695 & 0.9356 & 0.8908 & 0.9140 & 0.5328 & 0.6551 & 0.7201 & 0.7480 \\ 
		LINE &
		0.6525 & 0.9323 & 0.9110 & 0.9263 & 0.7698 & 0.8989 & 0.8659 & 0.8853 & 0.5261 & 0.6095 & 0.7209 & 0.7251 \\ 
		PTE &
		0.6426 & 0.9057 & 0.5723 & 0.5732 & 0.7607 & 0.7099 & 0.6958 & 0.7092 & 0.5292 & 0.6040 & 0.5836 & 0.5935 \\
		\midrule
		Metapath2vec-$\mathcal P_{1}$ &
        0.6202 & 0.7481 & 0.7412 & 0.7454 & 0.8178 & 0.9872 & 0.9955 & 0.9941 & -- & -- & -- & -- \\
		Metapath2vec-$\mathcal P_{2}$ &
		0.6246 & 0.7733 & 0.7715 & 0.7873 & -- & -- & -- & -- & 0.5428 & 0.7575 & 0.8027 & {\bf 0.8200} \\ 
		\hline
		Metagraph2vec-$\mathcal S_{1}$ &
	    0.6362 & 0.7450 & 0.7580 & 0.7635 & 0.7948 & 0.9814 & 0.9892 & 0.9919 & -- & -- & -- & -- \\ 
		Metagraph2vec-$\mathcal S_{2}$ &
		0.6430 & 0.7536 & 0.7573 & 0.7714 & 0.8072 & 0.9900 & 0.9946 & 0.9950 & 0.5500 & 0.6838 & 0.7496 & 0.7627 \\
		\midrule
		SpaceyMetapath-$\mathcal P_{1}$ &
		0.6329 & 0.7558 & 0.7498 & 0.7559 & {\bf 0.8217} & 0.9915 & 0.9979 & 0.9973 & -- & -- & -- & -- \\ 
		SpaceyMetapath-$\mathcal P_{2}$ &
		0.6392 & 0.7723 & 0.7721 & 0.7891 & -- & -- & -- & -- & {\bf 0.5590} & {\bf 0.7594} & {\bf 0.8075} & 0.8199 \\
		\hline
		SpaceyMetagraph-$\mathcal S_{1}$ &
		0.6416 & 0.7491 & 0.7607 & 0.7655 & 0.7991 & 0.9865 & 0.9915 & 0.9936 & -- & -- & -- & -- \\
		SpaceyMetagraph-$\mathcal S_{2}$ &
		0.6457 & 0.7618 & 0.7542 & 0.7713 & 0.8157 & {\bf 0.9962} & {\bf 0.9990} & {\bf 0.9982} & 0.5497 & 0.6858 & 0.7541 & 0.7662 \\
		\hline
		SpaceyMetaschema &
		{\bf 0.7187} & {\bf 0.9874} & {\bf 0.9943} & {\bf 0.9947} & 0.7983 & 0.9856 & 0.9848 & 0.9853 & 0.5387 & 0.6828 & 0.7242 & 0.7466 \\
		\bottomrule
	\end{tabular}
%	\vspace{-0.1in}
\end{table*}

\begin{table*}[t]
	 	\small
%		\footnotesize
	\caption{\small The AUC scores for link prediction on the DBLP dataset. The binary operators: (a) Average, (b) Hadamard, (c)
		Weighted-L1, and (d) Weighted-L2. % are defined in Table~\ref{Tab:binary_operators}. 
		``--'' indicates that the used meta-path/meta-graph cannot generate embeddings for nodes of target type.}\label{Tab:lp_results_DBLP_in_appendix}
	\vspace{-0.1in}
	\centering
	\begin{tabular}{p{2.8cm}<{\centering}|p{0.8cm}<{\centering}|p{0.8cm}<{\centering}|p{0.8cm}<{\centering}|p{0.8cm}<{\centering}|p{0.8cm}<{\centering}|p{0.8cm}<{\centering}|p{0.8cm}<{\centering}|p{0.8cm}<{\centering}|p{0.8cm}<{\centering}|p{0.8cm}<{\centering}|p{0.8cm}<{\centering}|p{0.8cm}<{\centering}}
		\toprule
		Edge Type & \multicolumn{4}{c|}{Paper--Author} & \multicolumn{4}{c|}{Paper--Conf.} & \multicolumn{4}{c}{Paper--Term} \\
		\midrule
		Operator & (a) & (b) & (c) & (d) & (a) & (b) & (c) & (d) & (a) & (b) & (c) & (d) \\
		\midrule
		DeepWalk &
0.5438 & 0.9750 & 0.9892 & 0.9893 & 0.8490 & 0.9710 & 0.9244 & 0.9432 & 0.7423 & 0.8233 & 0.9718 & 0.9734 \\
		LINE &
0.5025 & 0.9323 & 0.9110 & 0.9263 & 0.7698 & 0.8989 & 0.8659 & 0.8853 & 0.6261 & 0.8095 & 0.7609 & 0.7951 \\  
		PTE &
0.5126 & 0.9057 & 0.5723 & 0.5732 & 0.7607 & 0.7099 & 0.6958 & 0.7092 & 0.5792 & 0.6040 & 0.5836 & 0.5935 \\
\midrule
		Metapath2vec-$\mathcal P_{1}$ &
0.5628 & 0.9741 & 0.9929 & 0.9907 & 0.8668 & 0.9809 & 0.9850 & 0.9802 & -- & -- & -- & -- \\
		Metapath2vec-$\mathcal P_{2}$ &
0.5493 & 0.9925 & 0.9985 & 0.9989 & -- & -- & -- & -- & 0.7407 & 0.8370 & 0.9894 & 0.9930 \\
\hline
		Metagraph2vec-$\mathcal S_{1}$ &
0.5671 & 0.9907 & 0.9983 & 0.9987 & 0.8600 & 0.9747 & 0.9670 & 0.9736 & -- & -- & -- & -- \\ 
		Metagraph2vec-$\mathcal S_{2}$ &
0.5825 & 0.9903 & 0.9985 & 0.9988 & 0.8663 & 0.9850 & 0.9845 & 0.9862 & 0.7520 & 0.8234 & 0.9599 & 0.9705 \\ 
\midrule
		SpaceyMetapath-$\mathcal P_{1}$ &
0.5792 & 0.9854 & 0.9981 & 0.9975 & 0.8718 & 0.9883 & 0.9900 & 0.9883 & -- & -- & -- & -- \\ 
		SpaceyMetapath-$\mathcal P_{2}$ &
0.5519 & {\bf 0.9974} & 0.9993 & {\bf 0.9995} & -- & -- & -- & -- & 0.7451 & {\bf 0.8401} & {\bf 0.9914} & {\bf 0.9939}\\
\hline 
		SpaceyMetagraph-$\mathcal S_{1}$ &
0.5737 & 0.9929 & 0.9990 & 0.9990 & 0.8676 & 0.9825 & 0.9742 & 0.9801 & -- & -- & -- & -- \\
		SpaceyMetagraph-$\mathcal S_{2}$ &
{\bf 0.5877} & 0.9962 & 0.9992 & 0.9993 & {\bf 0.8751} & 0.9906 & 0.9913 & 0.9903 & {\bf 0.7573} & 0.8246 & 0.9701 & 0.9799 \\
\hline
		SpaceyMetaschema &
0.5525 & 0.9957 & {\bf 0.9994} & 0.9992 & 0.8716 & {\bf 0.9962} & {\bf 0.9969} & {\bf 0.9974} & 0.7437 & 0.8296 & 0.9748 & 0.9816 \\
		\bottomrule
	\end{tabular}
%	\vspace{-0.1in}
\end{table*}

\begin{table*}[t]
	 	\small
%		\footnotesize
	\caption{\small The AUC scores for link prediction on the Douban dataset. The binary operators: (a) Average, (b) Hadamard, (c)
		Weighted-L1, and (d) Weighted-L2. %are defined in Table~\ref{Tab:binary_operators}. 
		``--'' indicates that the used meta-path/meta-graph cannot generate embeddings for nodes of target type.}\label{Tab:lp_results_Douban_in_appendix}
	\vspace{-0.1in}
	\centering
	\begin{tabular}{p{2.8cm}<{\centering}|p{0.8cm}<{\centering}|p{0.8cm}<{\centering}|p{0.8cm}<{\centering}|p{0.8cm}<{\centering}|p{0.8cm}<{\centering}|p{0.8cm}<{\centering}|p{0.8cm}<{\centering}|p{0.8cm}<{\centering}|p{0.8cm}<{\centering}|p{0.8cm}<{\centering}|p{0.8cm}<{\centering}|p{0.8cm}<{\centering}}
		\toprule
		Edge Type & \multicolumn{4}{c|}{User--User} & \multicolumn{4}{c|}{User--Movie} & \multicolumn{4}{c}{Movie--Director} \\
		\midrule
		Operator & (a) & (b) & (c) & (d) & (a) & (b) & (c) & (d) & (a) & (b) & (c) & (d) \\
		\midrule
		DeepWalk &
		0.6554 & 0.6001 & 0.6212 & 0.6251 & 0.7639 & 0.7238 & 0.8327 & 0.8419 & 0.6012 & 0.9399 & 0.9065 & 0.9111 \\ 
		LINE &
		0.6954 & 0.6125 & 0.6282 & 0.6133 & 0.7653 & 0.7133 & 0.8251 & 0.8361 & 0.5997 & 0.8906 & 0.8650 & 0.8724 \\
		PTE &
		0.7652 & 0.7516 & 0.5794 & 0.5802 & 0.6671 & 0.6092 & 0.6544 & 0.6535 & 0.5205 & 0.5976 & 0.6169 & 0.6175 \\ 
		\midrule
		Metapath2vec-$\mathcal P_{1}$ &
		0.6303 & 0.5572 & 0.6132 & 0.6236 & 0.7612 & 0.6567 & 0.8866 & 0.8930 & -- & -- & -- & -- \\
		Metapath2vec-$\mathcal P_{2}$ &
		0.6294 & 0.5558 & 0.6074 & 0.6096 & 0.8146 & 0.6480 & 0.8881 & 0.8888 & 0.6026 & 0.9847 & 0.9622 & 0.9676 \\ 
		\hline
		Metagraph2vec-$\mathcal S_{1}$ &
		0.6389 & 0.5649 & 0.6155 & 0.6194 & 0.7603 & 0.6734 & 0.8976 & 0.9011 & 0.6064 & 0.9911 & 0.9804 & 0.9849 \\ 
		Metagraph2vec-$\mathcal S_{2}$ &
		0.7097 & 0.6487 & 0.6609 & 0.6719 & 0.7633 & 0.6565 & 0.8246 & 0.8399 & 0.6073 & 0.9922 & 0.9228 & 0.9273 \\ 
		\midrule
		SpaceyMetapath-$\mathcal P_{1}$ &
		0.6427 & 0.5863 & 0.6229 & 0.6304 & 0.7936 & 0.6961 & 0.9149 & 0.9225 & -- & -- & -- & -- \\ 
		SpaceyMetapath-$\mathcal P_{2}$ &
		0.6364 & 0.5794 & 0.6221 & 0.6231 & 0.8237 & 0.6775 & 0.9094 & 0.9135 & 0.6145 & 0.9942 & 0.9892 & 0.9924 \\
		\hline
		SpaceyMetagraph-$\mathcal S_{1}$ &
		0.6456 & 0.5901 & 0.6254 & 0.6349 & 0.7962 & 0.6960 & {\bf 0.9187} & {\bf 0.9248} & 0.6181 & 0.9950 & {\bf 0.9979} & {\bf 0.9980} \\
		SpaceyMetagraph-$\mathcal S_{2}$ &
		0.7231 & 0.6778 & 0.6754 & 0.6850 & 0.7835 & 0.6750 & 0.8671 & 0.8787 & 0.6184 & {\bf 0.9954} & 0.9944 & 0.9953 \\ 
		\hline
		SpaceyMetaschema &
		{\bf 0.8006} & {\bf 0.9863} & {\bf 0.9748} & {\bf 0.9737} & {\bf 0.8554} & {\bf 0.8250} & 0.9027 & 0.9104 & {\bf 0.6215} & 0.9905 & 0.9971 & 0.9967 \\ 
		\bottomrule
	\end{tabular}
%	\vspace{-0.1in}
\end{table*}

\begin{table*}[t]
	 	\small
%		\footnotesize
	\caption{\small The AUC scores for link prediction on the Yelp dataset. The binary operators: (a) Average, (b) Hadamard, (c)
		Weighted-L1, and (d) Weighted-L2. % are defined in Table~\ref{Tab:binary_operators}. 
		``--'' indicates that the used meta-path/meta-graph cannot generate embeddings for nodes of target type.}\label{Tab:lp_results_Yelp_in_appendix}
	\vspace{-0.1in}
	\centering
	\begin{tabular}{p{2.8cm}<{\centering}|p{0.8cm}<{\centering}|p{0.8cm}<{\centering}|p{0.8cm}<{\centering}|p{0.8cm}<{\centering}|p{0.8cm}<{\centering}|p{0.8cm}<{\centering}|p{0.8cm}<{\centering}|p{0.8cm}<{\centering}|p{0.8cm}<{\centering}|p{0.8cm}<{\centering}|p{0.8cm}<{\centering}|p{0.8cm}<{\centering}}
		\toprule
		Edge Type & \multicolumn{4}{c|}{User--User} & \multicolumn{4}{c|}{User--Business} & \multicolumn{4}{c}{Business--City} \\
		\midrule
		Operator & (a) & (b) & (c) & (d) & (a) & (b) & (c) & (d) & (a) & (b) & (c) & (d) \\
		\midrule
		DeepWalk &
		0.8580 & 0.8926 & 0.8716 & 0.8851 & 0.7664 & 0.8428 & 0.9520 & 0.9647 & 0.8202 & 0.9120 & 0.9787 & 0.9740 \\ 
		LINE &
		0.8614 & 0.8958 & 0.8694 & 0.8815 & 0.7419 & 0.8448 & 0.9114 & 0.9198 & 0.8018 & 0.8988 & 0.9616 & 0.9631 \\ 
		PTE &
		0.8552 & 0.9004 & 0.7830 & 0.7890 & 0.7331 & 0.8253 & 0.8145 & 0.8147 & 0.7631 & 0.8176 & 0.8603 & 0.8565 \\
		\midrule
		Metapath2vec-$\mathcal P_{1}$ &
		0.6900 & 0.5785 & 0.6564 & 0.6608 & 0.6810 & 0.7978 & 0.9330 & 0.9410 & 0.8138 & 0.8876 & 0.9887 & 0.9815 \\
		Metapath2vec-$\mathcal P_{2}$ &
		0.7887 & 0.6357 & 0.7500 & 0.7588 & 0.6576 & 0.7613 & 0.8598 & 0.8577 & -- & -- & -- & -- \\ 
		\hline
		Metagraph2vec-$\mathcal S_{1}$ &
		0.6933 & 0.5901 & 0.6525 & 0.6615 & 0.6655 & 0.8507 & 0.9724 & 0.9772 & 0.8052 & 0.8672 & 0.9804 & 0.9794 \\ 
		Metagraph2vec-$\mathcal S_{2}$ &
		0.7715 & 0.6332 & 0.6737 & 0.6891 & 0.6789 & 0.8565 & 0.9731 & 0.9785 & -- & -- & -- & -- \\ 
		\midrule
		SpaceyMetapath-$\mathcal P_{1}$ &
		0.7194 & 0.5922 & 0.6756 & 0.6802 & 0.6855 & 0.8440 & 0.9437 & 0.9528 & 0.8252 & 0.9361 & {\bf 0.9960} & 0.9912 \\ 
		SpaceyMetapath-$\mathcal P_{2}$ &
		0.8090 & 0.6659 & 0.7614 & 0.7665 & 0.6766 & 0.8543 & 0.9332 & 0.9424 & -- & -- & -- & -- \\ 
		\hline
		SpaceyMetagraph-$\mathcal S_{1}$ &
		0.6948 & 0.5906 & 0.6608 & 0.6686 & 0.7157 & 0.8702 & 0.9737 & 0.9797 & 0.8216 & 0.9007 & 0.9887 & 0.9857 \\
		SpaceyMetagraph-$\mathcal S_{2}$ &
		0.7747 & 0.6455 & 0.6781 & 0.6922 & 0.7134 & 0.8773 & {\bf 0.9757} & {\bf 0.9809} & -- & -- & -- & -- \\
		\hline 
		SpaceyMetaschema &
		{\bf 0.8725} & {\bf 0.9057} & {\bf 0.9585} & {\bf 0.9650} & {\bf 0.8015} & {\bf 0.8800} & 0.9496 & 0.9570 & {\bf 0.8462} & {\bf 0.9613} & {\bf 0.9960} & {\bf 0.9954} \\
		\bottomrule
	\end{tabular}
%	\vspace{-0.1in}
\end{table*}
